# Supplementary material for: Superexchange interactions and magnetic anisotropy in MnPSe$_3$ monolayer
Source: arXiv:2401.16154 source file (2024-01-29)
Supplement: Supplementary file 1 [file MnPSe3_CPL_SM.pdf]

Supplemental Materials for

Superexchange interactions and magnetic anisotropy in MnPSe<sub>3</sub>  
monolayer

Guangyu Wang,<sup>1, 2, \*</sup> Ke Yang,<sup>3, 1, \*</sup> Yaozhenghang Ma,<sup>1, 2</sup> Lu Liu,<sup>1, 2</sup> Di Lu,<sup>1, 2</sup>, Yuxuan Zhou,<sup>1, 2</sup>  
and Hua Wu<sup>1, 2, 4, †</sup>

<sup>1</sup> Laboratory for Computational Physical Sciences (MOE), State Key Laboratory of Surface Physics, and Department of Physics, Fudan University, Shanghai 200433, China

<sup>2</sup> Shanghai Qi Zhi Institute, Shanghai 200232, China

<sup>3</sup> College of Science, University of Shanghai for Science and Technology, Shanghai 200093, China

<sup>4</sup> Collaborative Innovation Center of Advanced Microstructures, Nanjing 210093, China

\* These authors contributed equally to this work.

†E-mail: wuh@fudan.edu.cn

## I. The magnetic exchange parameters

The value of  $J = 1.41$  meV in the main text is obtained by considering only the first nearest neighboring magnetic coupling, i.e., the spin Hamiltonian is given by

$$H = \sum_{i,j} \frac{J}{2} \vec{S}_i \vec{S}_j + \sum_i \{D(S_i^c)^2 + E_n[(S_i^b)^2 - (S_i^a)^2]\}$$

where  $D$  and  $E_n$  are the magnetic anisotropy parameters. In this case, the calculated magnetic specific heat from our Monte Carlo simulations shows  $T_N = 47$  K, which agrees well with the experimental 40 K.

We also compute the 1st, 2nd, and 3rd nearest neighboring magnetic couplings  $J_1$ ,  $J_2$  and  $J_3$ , using the supercells and four different magnetic states in Figs. S1 and S2. The spin Hamiltonian in this case is given by

$$H = \sum_{k=1,2,3} \sum_{i,j} \frac{J_k}{2} \vec{S}_i \vec{S}_j + \sum_i \{D(S_i^c)^2 + E_n[(S_i^b)^2 - (S_i^a)^2]\}.$$

Counting  $JS^2$  for each spin pair, the magnetic exchange energies (per formula unit) of the four magnetic states are written as follows

$$E_{FM} = (\frac{3}{2}J_1 + 3J_2 + \frac{3}{2}J_3)S^2$$

$$E_{Neel} = (-\frac{3}{2}J_1 + 3J_2 - \frac{3}{2}J_3)S^2$$

$$E_{Stripy} = (-\frac{1}{2}J_1 - J_2 + \frac{3}{2}J_3)S^2$$

$$E_{Zigzag} = (\frac{1}{2}J_1 - J_2 - \frac{3}{2}J_3)S^2$$

The relative total energy results are shown in Table S1. Using those values and the above equations, we can calculate  $J_1 = 0.88$  meV,  $J_2 = 0.08$  meV, and  $J_3 = 0.54$  meV.

Table S1. Relative total energies  $\Delta E$  (meV/fu) for MnPSe<sub>3</sub> monolayer by GGA+ $U$ . The calculated three AF exchange parameters (meV) are listed.

| States     | FM           | AF-Néel      | AF-Stripy    | AF-Zigzag |
|------------|--------------|--------------|--------------|-----------|
| $\Delta E$ | 26.4         | 0            | 13.6         | 9.0       |
|            | $J_1 = 0.88$ | $J_2 = 0.08$ | $J_3 = 0.54$ |           |

In the honeycomb structure of MnPSe<sub>3</sub> monolayer, the joint contribution of  $J_1$  and  $J_3$  ( $J_1 + J_3 = 1.42$  meV) is equivalent to the exchange parameter  $J = 1.41$  meV in the main text. With inclusion of the small  $J_2$  but its higher six-coordination than three-coordination for  $J_1$  and  $J_3$ ,  $T_N$  is somewhat increased to 53 K, from 47 K according to the Monte Carlo simulation using  $J = 1.41$  meV in the main text. Nevertheless, either 47 K or 53 K is in reasonable agreement with the experimental 40 K. Therefore, for the convenience of discussion, we assume the AF exchange parameter is 1.41 meV, as mentioned in the main text.

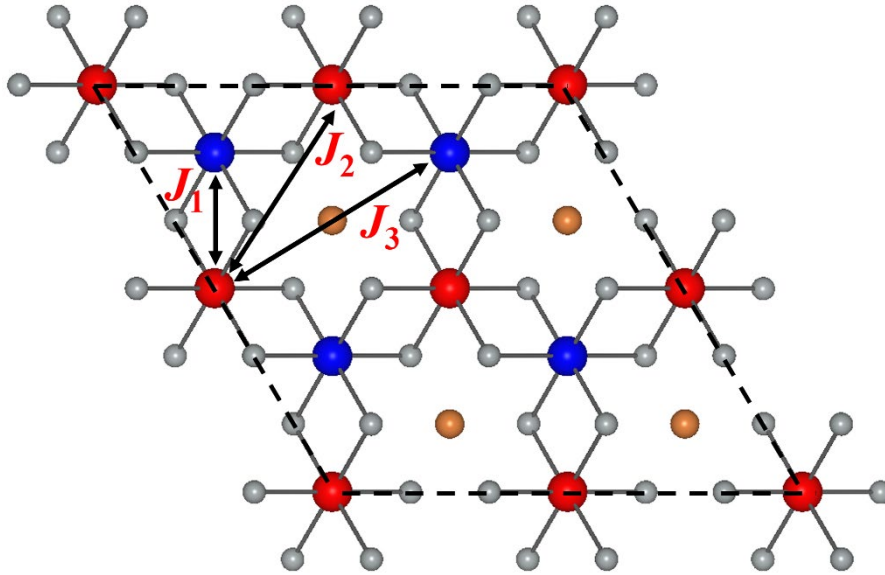

Fig. S1: The first ( $J_1$ ), second ( $J_2$ ) and third ( $J_3$ ) nearest neighbor exchange interactions.

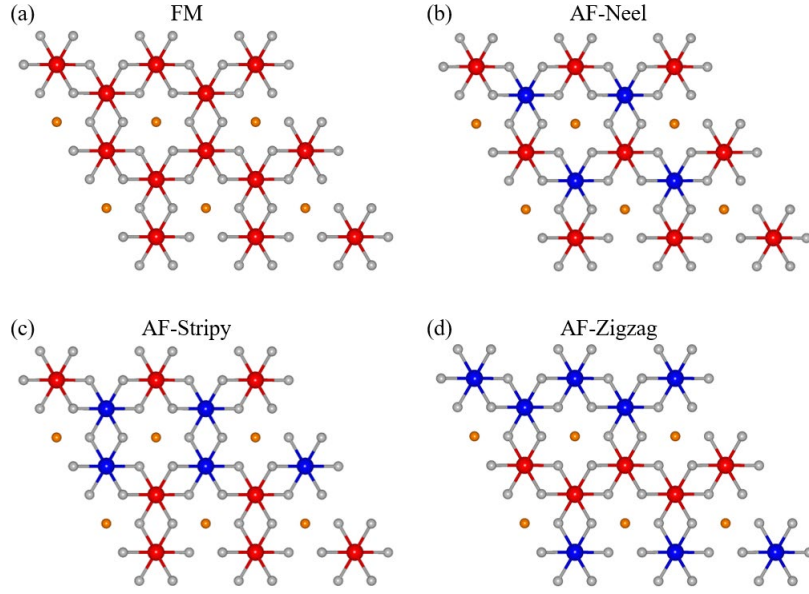

Fig. S2: Four different magnetic structures: (a) FM, (b) AF-Néel, (c) AF-Stripy, and (d) AF-Zigzag. Up (down) spins are represented by red (blue) balls.

## II. Hopping integrals of spin-up channels

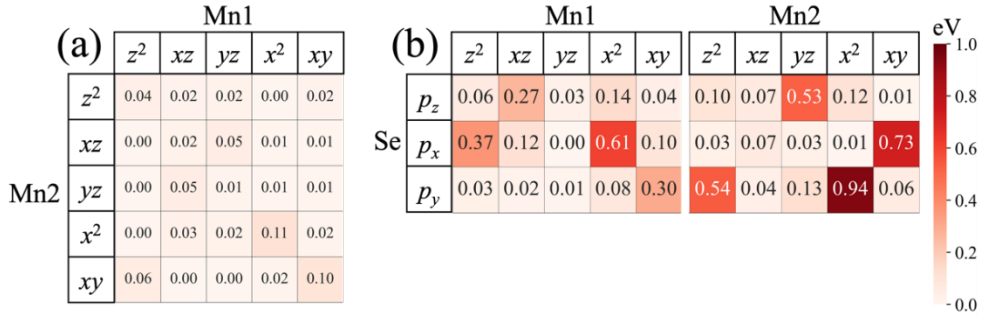

Fig. S3: (a): Hopping integrals of spin-up channels calculated by MLWFs basis set between 3d orbitals of Mn1 and Mn2. (b): Hopping integrals of spin-up channels between 3d orbitals of Mn and 4p orbitals of Se.

## III. The distributions of MAE in the reciprocal space in the FM state

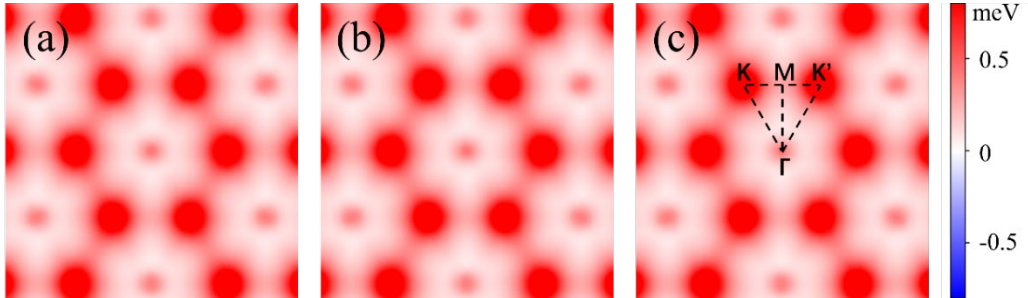

Fig. S4: The distributions of MAE in the reciprocal space in the FM MnPSe<sub>3</sub> monolayer. (a):  $E^c - E^a$ , (b):  $E^{-c} - E^{-a}$ , (c):  $((E^c - E^a) + (E^{-c} - E^{-a}))/2$ .

#### IV. Polar diagrams of MAE

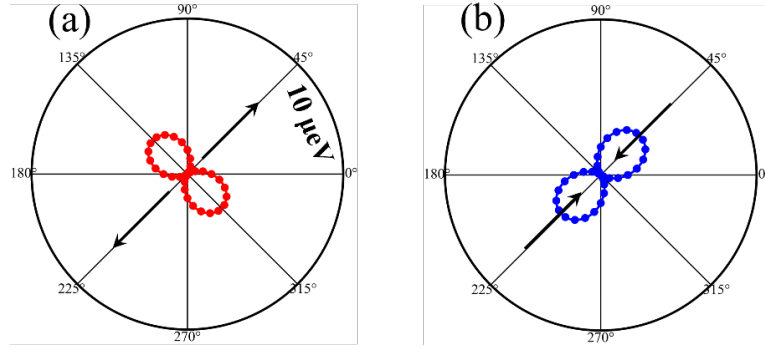

Fig. S5: (a): Polar diagrams of the MAE in the  $ab$  plane. The  $\text{MnPSe}_3$  monolayer is under 2% uniaxial tensile strain with strain direction along 45° with respect to the  $a$  axis. (b):  $\text{MnPSe}_3$  monolayer is under 2% uniaxial compressive strain with strain direction along 45° with respect to the  $a$  axis.

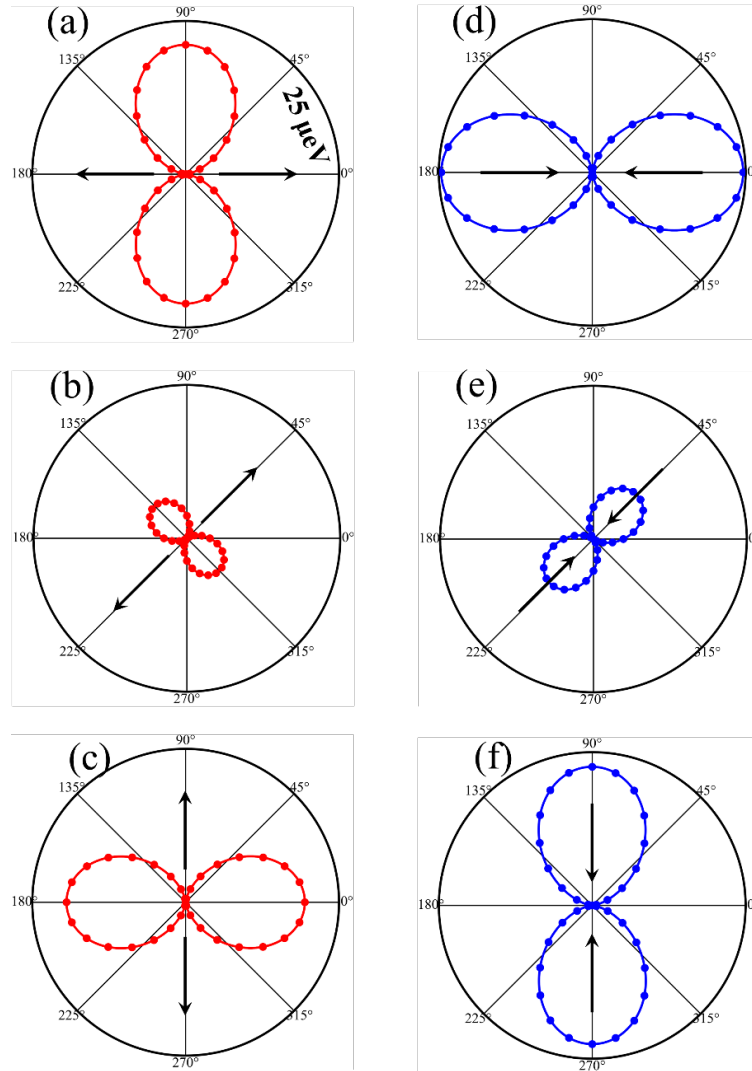

Fig. S6: Polar diagrams of the MAE in the  $ab$  plane. The  $\text{MnPSe}_3$  monolayer is under 5% uniaxial tensile strain (a-c) and compressive strain (d-f).
